# Supplementary material for: Revisiting Nonlocal Self-Similarity from Continuous Representation
Source: arXiv:2401.00708 source file (2024-01-01)
Supplement: Supplementary file 1 [file supplementary.pdf]

# Supplementary Material of "Revisiting Nonlocal Self-Similarity from Continuous Representation"

Yisi Luo, Xile Zhao, *Member, IEEE*, Deyu Meng, *Member, IEEE*

## I. PROOF OF LEMMA 2

**Definition 1** (Sampled tensor set of a function [1]). *For a multivariate function $h_l(\cdot):\Omega\to\mathbb{R}$, where $\Omega=\Omega_1\times\Omega_2\times\cdots\times\Omega_{N+1}\subset\mathbb{R}^{N+1}$ and $\Omega_d\subset\mathbb{R}$ $(d=1,\cdots,N+1)$, we define the sampled tensor set $S[h_l]$ as*

$$S[h_l]:=\{\mathcal{T}:\mathcal{T}_{(i_1,i_2,\cdots,i_{N+1})}=h_l(\mathbf{x}_{1_{(i_1)}},\mathbf{x}_{2_{(i_2)}},\cdots,\mathbf{x}_{N+1_{(i_{N+1})}}),\mathbf{x}_d\in\Omega_d^{n_d},n_d\in\mathbb{N}_+,d=1,2,\cdots,N+1\}. \quad (1)$$

*Here, $\mathbf{x}_d$ $(d=1,2,\cdots,N+1)$ denote the coordinate vector variables along the dimension $d$ and $n_d$ $(d=1,2,\cdots,N+1)$ are positive integer variables that determine the sizes of the sampled tensor $\mathcal{T}\in\mathbb{R}^{n_1\times n_2\times\cdots\times n_{N+1}}$.*

**Definition 2** (Function rank [1]). *Given a tensor function $h_l(\cdot):\Omega=\Omega_1\times\Omega_2\times\cdots\times\Omega_{N+1}\to\mathbb{R}$, we define a measure of its complexity, denoted by* F-rank$[h_l]$ *(function rank of $h_l(\cdot)$), as the supremum of Tucker rank [2] in the sampled tensor set $S[h_l]$:*

$$\text{F-rank}[h_l]:=(r_1,r_2,\cdots,r_{N+1}),\ \text{where } r_d=\sup_{\mathcal{T}\in S[h_l]}\text{rank}(\mathbf{T}^{(d)}), \quad (2)$$

*where $\mathbf{T}^{(d)}$ $(d=1,2,\cdots,N+1)$ denote the mode-$d$ unfolding matrices of $\mathcal{T}$ [2].*

**Lemma 2.** *(Low-rank tensor function factorization) Let $h_l(\cdot):\Omega\to\mathbb{R}$ be a bounded multivariate function, where $\Omega=\Omega_1\times\Omega_2\times\cdots\times\Omega_{N+1}\subset\mathbb{R}^{N+1}$ is the definition domain. Then:*

(i) *(Existence of low-rank tensor function factorization) If* F-rank$[h_l]=(r_1,r_2,\cdots,r_{N+1})$, *then there exist a core tensor $\mathcal{C}\in\mathbb{R}^{r_1\times r_2\times\cdots\times r_{N+1}}$ and $N+1$ bounded factor functions $f_1(\cdot):\Omega_1\to\mathbb{R}^{r_1}$, $f_2(\cdot):\Omega_2\to\mathbb{R}^{r_2}$,$\cdots$, $f_{N+1}(\cdot):\Omega_{N+1}\to\mathbb{R}^{r_{N+1}}$ such that for any $\mathbf{v}\in\Omega$, $h_l(\mathbf{v})=\mathcal{C}\times_1 f_1(\mathbf{v}_{(1)})\times_2 f_2(\mathbf{v}_{(2)})\times_3\cdots\times_{N+1}f_{N+1}(\mathbf{v}_{(N+1)})$.*

(ii) *(Low-rankness guarantee of the tensor function factorization) Let $\mathcal{C}\in\mathbb{R}^{r_1\times r_2\times\cdots\times r_{N+1}}$ be an arbitrary tensor and $f_1(\cdot):\Omega_1\to\mathbb{R}^{r_1}$, $f_2(\cdot):\Omega_2\to\mathbb{R}^{r_2}$,$\cdots$, $f_{N+1}(\cdot):\Omega_{N+1}\to\mathbb{R}^{r_{N+1}}$ be $N+1$ arbitrary bounded factor functions. Then we have $(\text{F-rank}[h_l])_{(d)}\le r_d$ $(d=1,2,\cdots,N+1)$, where $h_l(\cdot):\Omega=\Omega_1\times\Omega_2\times\cdots\times\Omega_{N+1}\to\mathbb{R}$ is defined by $h_l(\mathbf{v})=\mathcal{C}\times_1 f_1(\mathbf{v}_{(1)})\times_2 f_2(\mathbf{v}_{(2)})\times_3\cdots\times_{N+1}f_{N+1}(\mathbf{v}_{(N+1)})$ for any $\mathbf{v}\in\Omega$.*

*Proof.* We first prove (i). The proof of (i) is divided into three steps.

Step 1. (Linear representation of mode-1 function) Suppose that F-rank$[h_l]=(r_1,r_2,\cdots,r_{N+1})$ with $r_d<\infty$ $(d=1,2,\cdots,N+1)$. Let

$$R_1:=\{\text{rank}(\mathbf{T}^{(1)}):\texttt{fold}_1(\mathbf{T}^{(1)})\in S[h_l]\}. \quad (3)$$

Then $r_1=\sup R_1$. We can see that $R_1$ is a closed set. Thus there exists $\mathcal{X}_1\in S[h_l]$ such that $\text{rank}(\mathbf{X}_1^{(1)})=r_1$. Similarly, there exist $\mathcal{X}_2,\mathcal{X}_3,\cdots,\mathcal{X}_{N+1}\in S[h_l]$ such that $\text{rank}(\mathbf{X}_2^{(2)})=r_2$, $\text{rank}(\mathbf{X}_3^{(3)})=r_3$, $\cdots$, $\text{rank}(\mathbf{X}_{N+1}^{(N+1)})=r_{N+1}$. Suppose the coordinate vectors of sampling $\mathcal{X}_1$ from $h_l(\cdot)$ are $\mathbf{x}_1^{\mathcal{X}_1}$, $\mathbf{x}_2^{\mathcal{X}_1}$, $\cdots$, $\mathbf{x}_{N+1}^{\mathcal{X}_1}$. Define the same coordinate vectors for $\mathcal{X}_2$, $\mathcal{X}_3$, $\cdots$, $\mathcal{X}_{N+1}$ (i.e., $\mathbf{x}_1^{\mathcal{X}_2},\mathbf{x}_2^{\mathcal{X}_2},\cdots,\mathbf{x}_{N+1}^{\mathcal{X}_2},\mathbf{x}_1^{\mathcal{X}_3},\mathbf{x}_2^{\mathcal{X}_3},\cdots,\mathbf{x}_{N+1}^{\mathcal{X}_3},\cdots,\mathbf{x}_1^{\mathcal{X}_{N+1}},\mathbf{x}_2^{\mathcal{X}_{N+1}},\cdots,\mathbf{x}_{N+1}^{\mathcal{X}_{N+1}}$), and consider their concatenations:

$$\begin{cases}\mathbf{x}_1=[\mathbf{x}_1^{\mathcal{X}_1},\mathbf{x}_1^{\mathcal{X}_2},\cdots,\mathbf{x}_1^{\mathcal{X}_{N+1}}]\in{\Omega_1}^{1\times n_1},\\ \mathbf{x}_2=[\mathbf{x}_2^{\mathcal{X}_1},\mathbf{x}_2^{\mathcal{X}_2},\cdots,\mathbf{x}_2^{\mathcal{X}_{N+1}}]\in{\Omega_2}^{1\times n_2},\\ \quad\cdots\\ \mathbf{x}_{N+1}=[\mathbf{x}_{N+1}^{\mathcal{X}_1},\mathbf{x}_{N+1}^{\mathcal{X}_2},\cdots,\mathbf{x}_{N+1}^{\mathcal{X}_{N+1}}]\in{\Omega_{N+1}}^{1\times n_{N+1}}.\end{cases} \quad (4)$$

Here we introduce $n_d$ $(d=1,2,\cdots,N+1)$ to denote the sizes of these vectors. Define the tensor $\mathcal{T}\in\mathbb{R}^{n_1\times n_2\times\cdots\times n_{N+1}}$ as

$$\mathcal{T}_{(i_1,i_2,\cdots,i_{N+1})}=h_l(\mathbf{x}_{1_{(i_1)}},\mathbf{x}_{2_{(i_2)}},\cdots,\mathbf{x}_{N+1_{(i_{N+1})}}),\ \forall\, i_1,i_2,\cdots,i_{N+1}. \quad (5)$$

It is easy to see that $\text{rank}_T(\mathcal{T})=(r_1,r_2,\cdots,r_{N+1})$. Each column of $\mathbf{T}^{(1)}$ is a mode-1 fiber of $\mathcal{T}$, so we can denote the $r_1$ column basis vectors of $\mathbf{T}^{(1)}$ by $\mathcal{T}_{(:,i_{2,1},\cdots,i_{N+1,1})},\mathcal{T}_{(:,i_{2,2},\cdots,i_{N+1,2})},\cdots,\mathcal{T}_{(:,i_{2,r_1},\cdots,i_{N+1,r_1})}$, where $i_{d,j}$ are some coordinate scalars $(d=2,3,\cdots,N+1,\ j=1,2,\cdots,r_1)$.

Now let us consider any $x_2\in\Omega_2,x_3\in\Omega_3,\cdots,x_{N+1}\in\Omega_{N+1}$. We define a new tensor $\mathcal{U}\in\mathbb{R}^{n_1\times(n_2+1)\times(n_3+1)\times\cdots\times(n_{N+1}+1)}$ as $\mathcal{U}_{(i_1,i_2,\cdots,i_{N+1})}=h_l(\mathbf{x}_{1_{(i_1)}},\mathbf{x}'_{2_{(i_2)}},\cdots,\mathbf{x}'_{N+1_{(i_{N+1})}})$, where $\mathbf{x}'_2=[\mathbf{x}_2,x_2],\cdots,\mathbf{x}'_{N+1}=[\mathbf{x}_{N+1},x_{N+1}]$ are concatenations

of vectors and scalars. Since $\mathcal{U} \in S[h_l]$, we have $\text{rank}(\mathbf{U}^{(1)}) \leq r_1$. Meanwhile, from the definition of $\mathcal{U}$ we see that $\mathbf{T}^{(1)}$ is a sub-matrix of $\mathbf{U}^{(1)}$, which deduces $r_1 = \text{rank}(\mathbf{T}^{(1)}) \leq \text{rank}(\mathbf{U}^{(1)})$. Thus we have $\text{rank}(\mathbf{U}^{(1)}) = \text{rank}(\mathbf{T}^{(1)}) = r_1$, and $\mathcal{T}_{(:,i_{2,1},\cdots,i_{N+1,1})}, \mathcal{T}_{(:,i_{2,2},\cdots,i_{N+1,2})}, \cdots, \mathcal{T}_{(:,i_{2,r_1},\cdots,i_{N+1,r_1})}$ are $r_1$ basis vectors of the column space of $\mathbf{U}^{(1)}$. Note that $\mathcal{U}_{(:,n_2+1,n_3+1,\cdots,n_{N+1}+1)}$ is a column of $\mathbf{U}^{(1)}$. Hence, it can be linearly represented by these basis vectors with a unique coefficient vector $\mathbf{c} \in \mathbb{R}^{r_1}$, i.e.,

$$\mathcal{U}_{(:,n_2+1,n_3+1,\cdots,n_{N+1}+1)} = \sum_{j=1}^{r_1} \mathbf{c}_{(j)} \mathcal{T}_{(:,i_{2,j},i_{3,j},\cdots,i_{N+1,j})}. \tag{6}$$

Meanwhile, from definition we see that $\mathcal{U}_{(i_1,n_2+1,\cdots,n_{N+1}+1)} = h_l(\mathbf{x}_{1_{(i_1)}}, x_2, \cdots, x_{N+1})$ for any $i_1 \in \{1, 2, \cdots, n_1\}$. Thus, the following equality holds:

$$h_l(\mathbf{x}_{1_{(i_1)}}, x_2, \cdots, x_{N+1}) = \sum_{j=1}^{r_1} \mathbf{c}_{(j)} \mathcal{T}_{(i_1,i_{2,j},i_{3,j},\cdots,i_{N+1,j})} \overset{(5)}{=} \sum_{j=1}^{r_1} \mathbf{c}_{(j)} h_l(\mathbf{x}_{1_{(i_1)}}, \mathbf{x}_{2_{(i_{2,j})}}, \cdots, \mathbf{x}_{N+1_{(i_{N+1,j})}}). \tag{7}$$

Next, we will generalize this conclusion from $\mathbf{x}_{1_{(i_1)}} \in \{\mathbf{x}_{1_{(1)}}, \mathbf{x}_{1_{(2)}}, \cdots, \mathbf{x}_{1_{(n_1)}}\}$ to any $x_1 \in \Omega_1$, i.e., we will show that

$$h_l(x_1, x_2, \cdots, x_{N+1}) = \sum_{j=1}^{r_1} \mathbf{c}_{(j)} h_l(x_1, \mathbf{x}_{2_{(i_{2,j})}}, \cdots, \mathbf{x}_{N+1_{(i_{N+1,j})}}) \tag{8}$$

holds for any $x_1 \in \Omega_1$.

Given any $x_1 \in \Omega_1$, consider the following tensor $\mathcal{M} \in \mathbb{R}^{(n_1+1)\times(n_2+1)\times\cdots\times(n_{N+1}+1)}$, where

$$\mathcal{M}_{(i_1,i_2,\cdots,i_{N+1})} = h_l(\mathbf{x}'_{1_{(i_1)}}, \mathbf{x}'_{2_{(i_2)}}, \cdots, \mathbf{x}'_{N+1_{(i_{N+1})}}) \tag{9}$$

and $\mathbf{x}'_1 = [\mathbf{x}_1, x_1]$. We can see that $\mathcal{M} \in S[h_l]$ and $\mathbf{T}^{(1)}$ is a sub-matrix of $\mathbf{M}^{(1)}$. Hence $\text{rank}(\mathbf{M}^{(1)}) = r_1$. It is easy to verify that $\mathcal{M}_{(:,i_{2,1},\cdots,i_{N+1,1})}, \mathcal{M}_{(:,i_{2,2},\cdots,i_{N+1,2})}, \cdots, \mathcal{M}_{(:,i_{2,r_1},\cdots,i_{N+1,r_1})}$ are $r_1$ basis vectors of $\mathbf{M}^{(1)}$ and $\mathcal{M}_{(:,n_2+1,n_3+1,\cdots,n_{N+1}+1)}$ is a column of $\mathbf{M}^{(1)}$. So it admits

$$\mathcal{M}_{(:,n_2+1,n_3+1,\cdots,n_{N+1}+1)} = \sum_{j=1}^{r_1} \mathbf{b}_{(j)} \mathcal{M}_{(:,i_{2,j},\cdots,i_{N+1,j})}, \tag{10}$$

where $\mathbf{b}$ is the coefficient vector. Hence $\mathcal{M}_{(1:n_1,n_2+1,n_3+1,\cdots,n_{N+1}+1)} = \sum_{j=1}^{r_1} \mathbf{b}_{(j)} \mathcal{M}_{(1:n_1,i_{2,j},\cdots,i_{N+1,j})}$. From the definition of $\mathcal{M}$ we see that $\mathcal{M}_{(1:n_1,n_2+1,n_3+1,\cdots,n_{N+1}+1)} = \mathcal{U}_{(:,n_2+1,n_3+1,\cdots,n_{N+1}+1)}$ and $\mathcal{M}_{(1:n_1,i_{2,j},\cdots,i_{N+1,j})} = \mathcal{T}_{(:,i_{2,j},\cdots,i_{N+1,j})}$ for any $j \in \{1, 2, \cdots, r_1\}$. Thus we have

$$\mathcal{U}_{(:,n_2+1,n_3+1,\cdots,n_{N+1}+1)} = \sum_{j=1}^{r_1} \mathbf{b}_{(j)} \mathcal{T}_{(:,i_{2,j},\cdots,i_{N+1,j})}. \tag{11}$$

From Eqs. (6), (11) and the uniqueness of the coefficient vector, we get that $\mathbf{b} = \mathbf{c}$. Hence, we have

$$\mathcal{M}_{(:,n_2+1,n_3+1,\cdots,n_{N+1}+1)} = \sum_{j=1}^{r_1} \mathbf{c}_{(j)} \mathcal{M}_{(:,i_{2,j},\cdots,i_{N+1,j})}, \tag{12}$$

by following Eq. (10). Note that

$$\begin{aligned} &\mathcal{M}_{(n_1+1,n_2+1,\cdots,n_{N+1}+1)} = h_l(x_1, x_2, \cdots, x_{N+1}), \\ &\mathcal{M}_{(n_1+1,i_{2,j},i_{3,j},\cdots,i_{N+1,j})} = h_l(x_1, \mathbf{x}_{2_{(i_{2,j})}}, \mathbf{x}_{3_{(i_{3,j})}}, \cdots, \mathbf{x}_{N+1_{(i_{N+1,j})}}), \end{aligned} \tag{13}$$

hence Eq. (8) is true for any $x_1 \in \Omega_1$. This gives the linear representation of the mode-1 function $h_l(x_1, x_2, \cdots, x_{N+1})$ (with fixed $x_2, x_3, \cdots, x_{N+1}$ and variable $x_1$) using basis functions $h_l(x_1, \mathbf{x}_{2_{(i_{2,j})}}, \mathbf{x}_{3_{(i_{3,j})}}, \cdots, \mathbf{x}_{N+1_{(i_{N+1,j})}})$ $(j = 1, 2, \cdots, r_1)$.

Step 2. (Mode-1 function factorization and F-rank invariance) We define the factor function $f_1(\cdot) : \Omega_1 \to \mathbb{R}^{r_1}$ as

$$\begin{aligned} f_1(x_1) := [&h_l(x_1, \mathbf{x}_{2_{(i_{2,1})}}, \mathbf{x}_{3_{(i_{3,1})}}, \cdots, \mathbf{x}_{N+1_{(i_{N+1,1})}}), h_l(x_1, \mathbf{x}_{2_{(i_{2,2})}}, \mathbf{x}_{3_{(i_{3,2})}}, \cdots, \mathbf{x}_{N+1_{(i_{N+1,2})}}), \cdots, \\ &h_l(x_1, \mathbf{x}_{2_{(i_{2,r_1})}}, \mathbf{x}_{3_{(i_{3,r_1})}}, \cdots, \mathbf{x}_{N+1_{(i_{N+1,r_1})}})] \in \mathbb{R}^{r_1}. \end{aligned} \tag{14}$$

Also, define the tensor function $h(\cdot) : \{1, 2, \cdots, r_1\} \times \Omega_2 \times \cdots \times \Omega_{N+1} \to \mathbb{R}$ as

$$h(i_1, x_2, \cdots, x_{N+1}) := (c(x_2, \cdots, x_{N+1}))_{(i_1)}, \tag{15}$$

where the mapping $c(x_2, \cdots, x_{N+1}) : \Omega_2 \times \cdots \times \Omega_{N+1} \to \mathbb{R}^{r_1}$ returns the coefficient vector $\mathbf{c}$ in Eq. (8) with the given coordinates $x_2 \in \Omega_2, \cdots, x_{N+1} \in \Omega_{N+1}$ (The coefficient vector $\mathbf{c}$ is depend on the coordinates $x_2, \cdots, x_{N+1}$). $(c(x_2, \cdots, x_{N+1}))_{(i_1)}$ denotes the $i_1$-th element of $c(x_2, \cdots, x_{N+1})$. From Step 1 we can see that for any $(x_1, x_2, \cdots, x_{N+1}) \in$

$\Omega = \Omega_1 \times \Omega_2 \times \cdots \times \Omega_{N+1}$, it holds that

$$h_l(x_1, x_2, \cdots, x_{N+1}) = \sum_{j=1}^{r_1} h(j, x_2 \cdots, x_{N+1}) \, (f_1(x_1))_{(j)}, \tag{16}$$

where $(f_1(x_1))_{(j)}$ denotes the $j$-th element of $f_1(x_1)$. It can be re-written in a tensor-matrix product form:

$$h_l(x_1, x_2, \cdots, x_{N+1}) = h(:, x_2, \cdots, x_{N+1}) \times_1 f_1(x_1), \tag{17}$$

where

$$h(:, x_2, \cdots, x_{N+1}) := [h(1, x_2, \cdots, x_{N+1}), h(2, x_2, \cdots, x_{N+1}), \cdots, h(r_1, x_2, \cdots, x_{N+1})]^T \in \mathbb{R}^{r_1 \times 1 \times \cdots \times 1}. \tag{18}$$

We call this factorization of $h_l(\cdot)$ as the mode-1 low-rank function factorization. Next, we will show that this factorization has F-rank invariant property, i.e., we will show that F-rank$[h_l]$ = F-rank$[h]$. First, it is easy to see that $(\text{F-rank}[h])_{(1)} \leq r_1$ since the definition domain of $h(\cdot)$ in the first dimension is $\{1, 2, \cdots, r_1\}$. Then, consider the tensor $\mathcal{H} \in \mathbb{R}^{r_1 \times n_2 \times \cdots \times n_{N+1}} \cap S[h]$ defined by $\mathcal{H}_{(i_1, i_2, \cdots, i_{N+1})} = h(i_1, \mathbf{x}_{2_{(i_2)}}, \cdots, \mathbf{x}_{N+1_{(i_{N+1})}})$. Also consider the matrix

$$\mathbf{U} = [f_1(\mathbf{x}_{1_{(1)}})^T, f_1(\mathbf{x}_{1_{(2)}})^T, \cdots, f_1(\mathbf{x}_{1_{(n_1)}})^T]^T \in \mathbb{R}^{n_1 \times r_1}. \tag{19}$$

Then we have $\mathcal{T} = \mathcal{H} \times_1 \mathbf{U}$, hence $\mathbf{T}^{(1)} = \mathbf{U}\mathbf{H}^{(1)}$, inducing that $r_1 = \text{rank}(\mathbf{T}^{(1)}) \leq \text{rank}(\mathbf{H}^{(1)})$. So we have $(\text{F-rank}[h])_{(1)} = r_1$. Next we show that $(\text{F-rank}[h])_{(2)} = r_2$. Define the matrix

$$\hat{\mathbf{U}} = \begin{pmatrix} \mathbf{U}^T & & & \\ & \mathbf{U}^T & & \\ & & \ddots & \\ & & & \mathbf{U}^T \end{pmatrix} \in \mathbb{R}^{r_1(n_3 n_4 \cdots n_{N+1}) \times n_1(n_3 n_4 \cdots n_{N+1})}. \tag{20}$$

We can see that $\mathbf{T}^{(2)} = \mathbf{H}^{(2)}\hat{\mathbf{U}}$. Hence, $r_2 = \text{rank}(\mathbf{T}^{(2)}) \leq \text{rank}(\mathbf{H}^{(2)})$, and thus $(\text{F-rank}[h])_{(2)} \geq r_2$. Consider any $\mathcal{A} \in \mathbb{R}^{m_1 \times m_2 \times \cdots \times m_{N+1}} \cap S[h]$. Suppose its corresponding coordinate vector along the first dimension is $\mathbf{x}_1^{\mathcal{A}} \in \{1, 2, \cdots, r_1\}^{m_1}$. Define the matrix

$$\mathbf{F} = \begin{pmatrix} \left(f_1(\mathbf{x}_{1_{(1)}})\right)_{\mathbf{x}^{\mathcal{A}}_{1_{(1)}}} & \left(f_1(\mathbf{x}_{1_{(1)}})\right)_{\mathbf{x}^{\mathcal{A}}_{1_{(2)}}} & \cdots & \left(f_1(\mathbf{x}_{1_{(1)}})\right)_{\mathbf{x}^{\mathcal{A}}_{1_{(m_1)}}} \\ \left(f_1(\mathbf{x}_{1_{(2)}})\right)_{\mathbf{x}^{\mathcal{A}}_{1_{(1)}}} & \left(f_1(\mathbf{x}_{1_{(2)}})\right)_{\mathbf{x}^{\mathcal{A}}_{1_{(2)}}} & \cdots & \left(f_1(\mathbf{x}_{1_{(2)}})\right)_{\mathbf{x}^{\mathcal{A}}_{1_{(m_1)}}} \\ \vdots & \vdots & \ddots & \vdots \\ \left(f_1(\mathbf{x}_{1_{(n_1)}})\right)_{\mathbf{x}^{\mathcal{A}}_{1_{(1)}}} & \left(f_1(\mathbf{x}_{1_{(n_1)}})\right)_{\mathbf{x}^{\mathcal{A}}_{1_{(2)}}} & \cdots & \left(f_1(\mathbf{x}_{1_{(n_1)}})\right)_{\mathbf{x}^{\mathcal{A}}_{1_{(m_1)}}} \end{pmatrix} \in \mathbb{R}^{n_1 \times m_1}. \tag{21}$$

Let $\mathcal{B} = \mathcal{A} \times_1 \mathbf{F}$, we can see that $\mathcal{B} \in S[h_l]$. Also, we have $\mathbf{B}^{(2)} = \mathbf{A}^{(2)}\hat{\mathbf{F}}$, where

$$\hat{\mathbf{F}} = \begin{pmatrix} \mathbf{F}^T & & & \\ & \mathbf{F}^T & & \\ & & \ddots & \\ & & & \mathbf{F}^T \end{pmatrix} \in \mathbb{R}^{m_1(m_3 m_4 \cdots m_{N+1}) \times n_1(m_3 m_4 \cdots m_{N+1})}. \tag{22}$$

From the definition of $f_1(\cdot)$, we can observe that $\mathbf{F}$ is full column rank, and thus $\hat{\mathbf{F}}$ is full row rank. Multiplying a full row rank matrix in the RHS does not change the rank. Therefore, $\text{rank}(\mathbf{B}^{(2)}) = \text{rank}(\mathbf{A}^{(2)})$ holds. Since $\mathcal{B} \in S[h_l]$, we have $\text{rank}(\mathbf{B}^{(2)}) \leq r_2$ and thus $\text{rank}(\mathbf{A}^{(2)}) \leq r_2$. Due to the arbitrariness of $\mathcal{A}$, we have $(\text{F-rank}[h])_{(2)} \leq r_2$, which deduces $(\text{F-rank}[h])_{(2)} = r_2$. In a similar way, we can show that $(\text{F-rank}[h])_3 = r_3, \cdots, (\text{F-rank}[h])_{N+1} = r_{N+1}$, which concludes the F-rank invariance of mode-1 low-rank function factorization.

Step 3. (Low-rank tensor function factorization) Now we have shown that F-rank$[h] = (r_1, r_2, \cdots, r_{N+1})$. Thus, similar to the mode-1 low-rank function factorization, $h(\cdot)$ can be factorized along mode-2, i.e., there exists a factor function $f_2(\cdot) : \Omega_2 \to \mathbb{R}^{r_2}$ and a tensor function $h_2(\cdot) : \{1, 2, \cdots, r_1\} \times \{1, 2, \cdots, r_2\} \times \Omega_3 \times \cdots \times \Omega_{N+1} \to \mathbb{R}$ such that

$$h(x_1, x_2, \cdots, x_{N+1}) = h_2(x_1, :, x_3, \cdots, x_{N+1}) \times_2 f_2(x_2) \tag{23}$$

holds for any $(x_1, x_2, \cdots, x_{N+1})$, where

$$\begin{aligned} h_2(x_1, :, x_3, \cdots, x_{N+1}) := [&h_2(x_1, 1, x_3, \cdots, x_{N+1}), h_2(x_1, 2, x_3, \cdots, x_{N+1}), \\ &\cdots, h_2(x_1, r_2, x_3, \cdots, x_{N+1})] \in \mathbb{R}^{1 \times r_2 \times 1 \times \cdots \times 1}. \end{aligned} \tag{24}$$

Similar to Step 2, we can show that $h_2(\cdot)$ is F-rank invariant, i.e., F-rank$[h_2] = (r_1, r_2, \cdots, r_{N+1})$. So we can apply

the same low-rank function factorization in mode-$d$ ($d = 3, 4, \cdots, N+1$) and get that there exist some factor functions $f_3(\cdot) : \Omega_3 \to \mathbb{R}^{r_3}, \cdots, f_{N+1}(\cdot) : \Omega_{N+1} \to \mathbb{R}^{r_{N+1}}$ and some tensor functions $h_d(\cdot) : \{1, 2, \cdots, r_1\} \times \{1, 2, \cdots, r_2\} \times \cdots \times \{1, 2, \cdots, r_d\} \times \Omega_{d+1} \times \cdots \times \Omega_{N+1} \to \mathbb{R}$ such that

$$h_d(x_1, x_2, \cdots, x_{N+1}) = h_{d+1}(x_1, x_2, \cdots, x_d, :, x_{d+2}, \cdots, x_{N+1}) \times_{d+1} f_{d+1}(x_{d+1}) \; (d = 2, 3, \cdots, N) \tag{25}$$

hold for any $(x_1, \cdots, x_{N+1})$. Finally, define the core tensor $\mathcal{C} \in \mathbb{R}^{r_1 \times r_2 \times \cdots \times r_{N+1}}$ by $\mathcal{C}_{(i_1, i_2 \cdots, i_{N+1})} = h_{N+1}(i_1, i_2, \cdots, i_{N+1})$ for any $(i_1, i_2, \cdots, i_{N+1})$. Then for any $(v_1, v_2, \cdots, v_{N+1}) \in \Omega$, we have

$$h_l(v_1, v_2, \cdots, v_{N+1}) = \mathcal{C} \times_{N+1} f_{N+1}(v_{N+1}) \times_N \cdots \times_2 f_2(v_2) \times_1 f_1(v_1). \tag{26}$$

One can verify that tensor-matrix product admits commutative law, which completes the proof of Lemma 2 (i).

Then, we prove Lemma 2 (ii). For any $\mathcal{G} \in S[h_l]$, suppose its sampling coordinate vectors are $\mathbf{x}_1^{\mathcal{G}} \in {\Omega_1}^{n_1}$, $\mathbf{x}_2^{\mathcal{G}} \in {\Omega_2}^{n_2}$, $\cdots$, $\mathbf{x}_{N+1}^{\mathcal{G}} \in {\Omega_{N+1}}^{n_{N+1}}$, i.e.,

$$\mathcal{G}_{(i_1, i_2, \cdots, i_{N+1})} = h_l(\mathbf{x}^{\mathcal{G}}_{1_{(i_1)}}, \mathbf{x}^{\mathcal{G}}_{2_{(i_2)}}, \cdots, \mathbf{x}^{\mathcal{G}}_{N+1_{(i_{N+1})}}), \; \forall \, i_1, i_2, \cdots, i_{N+1}. \tag{27}$$

Define the factor matrices

$$\begin{cases} \mathbf{U}_1 = (f_1(\mathbf{x}^{\mathcal{G}}_{1_{(1)}}), f_1(\mathbf{x}^{\mathcal{G}}_{1_{(2)}}), \cdots, f_1(\mathbf{x}^{\mathcal{G}}_{1_{(n_1)}}))^T \in \mathbb{R}^{n_1 \times r_1}, \\ \mathbf{U}_2 = (f_2(\mathbf{x}^{\mathcal{G}}_{2_{(1)}}), f_2(\mathbf{x}^{\mathcal{G}}_{2_{(2)}}), \cdots, f_2(\mathbf{x}^{\mathcal{G}}_{2_{(n_2)}}))^T \in \mathbb{R}^{n_2 \times r_2}, \\ \quad \cdots \\ \mathbf{U}_{N+1} = (f_{N+1}(\mathbf{x}^{\mathcal{G}}_{N+1_{(1)}}), f_{N+1}(\mathbf{x}^{\mathcal{G}}_{N+1_{(2)}}), \cdots, f_{N+1}(\mathbf{x}^{\mathcal{G}}_{N+1_{(n_{N+1})}}))^T \in \mathbb{R}^{n_{N+1} \times r_{N+1}}, \end{cases} \tag{28}$$

Then we have $\mathcal{G} = \mathcal{C} \times_1 \mathbf{U}_1 \times_2 \mathbf{U}_2 \times_3 \cdots \times_{N+1} \mathbf{U}_{N+1}$. Hence $(\text{rank}_T(\mathcal{G}))_{(d)} \leq r_d$ ($d = 1, 2, \cdots, N+1$). Thus we have $(\text{F-rank}[h_l])_{(d)} \leq r_d$ ($d = 1, 2, \cdots, N+1$). □

## II. Proof of Lemma 3

**Lemma 3.** *Let $\{\mathcal{C}_l\}_{l=1}^L$ be some bounded core tensors, and $f_{\theta_1}(\cdot)$, $f_{\theta_2}(\cdot)$,$\cdots$, $f_{\theta_{N+1}}(\cdot)$ be $N+1$ fully-connected neural networks with sine activation function $\sin(\omega \, \cdot)$ and depth $M$. Suppose that $\eta \in \mathbb{R}$ is an upper bound of the $\ell_1$-norm of core tensors and weight matrices of neural networks. Define the following coupled low-rank functions for $L$ continuous groups:*

$$s_l(\mathbf{v}) := \mathcal{C}_l \times_1 f_{\theta_1}(\mathbf{v}_{(1)}) \times_2 \cdots \times_{N+1} f_{\theta_{N+1}}(\mathbf{v}_{(N+1)}) : \mathbb{R}^{N+1} \to \mathbb{R}, \; l = 1, 2, \cdots, L. \tag{29}$$

*Then the following inequality is true for any two groups $l_1, l_2 \in \{1, 2, \cdots, L\}$, any dimension $d \in \{1, 2, \cdots, N+1\}$, and any two coordinates $v'_d, v''_d \in \mathbb{R}$ :*

$$|s_{l_1}(v_1, v_2, \cdots, v'_d, \cdots, v_{N+1}) - s_{l_2}(v_1, v_2, \cdots, v''_d, \cdots, v_{N+1})| \leq \delta_1 |v'_d - v''_d| + \delta_2, \tag{30}$$

*where*

$$\begin{aligned} &\delta_1 = \eta^{MN+M+1} \omega^{(M-1)(N+1)} \xi^N, \\ &\delta_2 = 2\eta^{MN+M+1} \omega^{(M-1)(N+1)} \xi^{N+1}, \\ &\xi = \max\{|v_1|, \cdots, |v'_d|, |v''_d|, \cdots, |v_{N+1}|\}. \end{aligned} \tag{31}$$

*When $l_1 = l_2$, the upper bound reduces to $\delta_1 |v'_d - v''_d|$.*

*Proof.* For any $l_1, l_2$, we directly calculate

$$\begin{aligned} &|s_{l_1}(v_1, v_2, \cdots, v'_d, \cdots, v_{N+1}) - s_{l_2}(v_1, v_2, \cdots, v''_d, \cdots, v_{N+1})| \\ =&|\mathcal{C}_{l_1} \times_1 f_{\theta_1}(v_1) \times_2 \cdots \times_d f_{\theta_d}(v'_d) \cdots \times_{N+1} f_{\theta_{N+1}}(v_{(N+1)}) \\ &\qquad - \mathcal{C}_{l_2} \times_1 f_{\theta_1}(v_{(1)}) \times_2 \cdots \times_d f_{\theta_d}(v''_d) \cdots \times_{N+1} f_{\theta_{N+1}}(v_{(N+1)})| \\ =&|(\mathcal{C}_{l_1} \times_d f_{\theta_d}(v'_d) - \mathcal{C}_{l_2} \times_d f_{\theta_d}(v''_d)) \times_1 f_{\theta_1}(v_1) \times_2 \cdots \times_{N+1} f_{\theta_{N+1}}(v_{N+1})| \\ \leq&\|(\mathcal{C}_{l_1} \times_d f_{\theta_d}(v'_d) - \mathcal{C}_{l_2} \times_d f_{\theta_d}(v''_d))\|_{\ell_1} \|f_{\theta_1}(v_1)\|_{\ell_1} \|f_{\theta_2}(v_2)\|_{\ell_1} \cdots \|f_{\theta_{N+1}}(v_{N+1})\|_{\ell_1} \\ =&\|(\mathcal{C}_{l_1} \times_d f_{\theta_d}(v'_d) - \mathcal{C}_{l_2} \times_d f_{\theta_d}(v'_d) + \mathcal{C}_{l_2} \times_d f_{\theta_d}(v'_d) - \mathcal{C}_{l_2} \times_d f_{\theta_d}(v''_d))\|_{\ell_1} \\ &\qquad \|f_{\theta_1}(v_1)\|_{\ell_1} \|f_{\theta_2}(v_2)\|_{\ell_1} \cdots \|f_{\theta_{N+1}}(v_{N+1})\|_{\ell_1} \\ \leq&(\|\mathcal{C}_{l_1} \times_d f_{\theta_d}(v'_d) - \mathcal{C}_{l_2} \times_d f_{\theta_d}(v'_d)\|_{\ell_1} + \|\mathcal{C}_{l_2} \times_d f_{\theta_d}(v'_d) - \mathcal{C}_{l_2} \times_d f_{\theta_d}(v''_d)\|_{\ell_1}) \\ &\qquad \|f_{\theta_1}(v_1)\|_{\ell_1} \|f_{\theta_2}(v_2)\|_{\ell_1} \cdots \|f_{\theta_{N+1}}(v_{N+1})\|_{\ell_1} \\ \leq&(\|\mathcal{C}_{l_1} - \mathcal{C}_{l_2}\|_{\ell_1} \|f_{\theta_d}(v'_d)\|_{\ell_1} + \|\mathcal{C}_{l_2}\|_{\ell_1} \|f_{\theta_d}(v'_d) - f_{\theta_d}(v''_d)\|_{\ell_1}) \|f_{\theta_1}(v_1)\|_{\ell_1} \|f_{\theta_2}(v_2)\|_{\ell_1} \cdots \|f_{\theta_{N+1}}(v_{N+1})\|_{\ell_1}. \end{aligned} \tag{32}$$

Note that $|\sin(\omega x)| \leq |\omega x|$ and it derives

$$\begin{aligned}\|f_{\theta_1}(v_1)\|_{\ell_1} =&\|\mathbf{H}_{1,M}(\sin(\omega\ \mathbf{H}_{1,M-1}\cdots\mathbf{H}_{1,2}(\sin(\omega\ \mathbf{H}_{1,1}v_1))))\|_{\ell_1}\\ \leq&\eta\|(\sin(\omega\ \mathbf{H}_{1,M-1}\cdots\mathbf{H}_{1,2}(\sin(\omega\ \mathbf{H}_{1,1}v_1))))\|_{\ell_1}\\ \leq&\eta\omega\|\mathbf{H}_{1,M-1}\cdots\mathbf{H}_{1,2}(\sin(\omega\ \mathbf{H}_{1,1}v_1))\|_{\ell_1}\leq\cdots\leq\eta^M\omega^{M-1}|v_1|,\end{aligned} \tag{33}$$

where $\{\mathbf{H}_{1,m}\}_{m=1}^M$ denote the weight matrices of the fully connected neural network $f_{\theta_1}(\cdot)$. Similarly we have $\|f_{\theta_d}(v_d)\|_{\ell_1} \leq \eta^M\omega^{M-1}|v_d|$ for any dimension $d$. Meanwhile,

$$\begin{aligned}\|f_{\theta_d}(v_d') - f_{\theta_d}(v_d'')\|_{\ell_1} &= \|\mathbf{H}_{d,M}(\sin(\omega\ \mathbf{H}_{d,M-1}\cdots\mathbf{H}_{d,2}(\sin(\omega\ \mathbf{H}_{d,1}v_d'))))\\ &\qquad - \mathbf{H}_{d,M}(\sin(\omega\ \mathbf{H}_{d,M-1}\cdots\mathbf{H}_{d,2}(\sin(\omega\ \mathbf{H}_{d,1}v_d''))))\|_{\ell_1}\\ &= \|\mathbf{H}_{d,M}(\sin(\omega\ \mathbf{H}_{d,M-1}\cdots\mathbf{H}_{d,2}(\sin(\omega\ \mathbf{H}_{d,1}v_d')))\\ &\qquad - \sin(\omega\ \mathbf{H}_{d,M-1}\cdots\mathbf{H}_{d,2}(\sin(\omega\ \mathbf{H}_{d,1}v_d''))))\|_{\ell_1}\\ &\leq \eta\|\sin(\omega\ \mathbf{H}_{d,M-1}\cdots\mathbf{H}_{d,2}(\sin(\omega\ \mathbf{H}_{d,1}v_d')))\\ &\qquad - \sin(\omega\ \mathbf{H}_{d,M-1}\cdots\mathbf{H}_{d,2}(\sin(\omega\ \mathbf{H}_{d,1}v_d'')))\|_{\ell_1}\\ &\leq \eta\omega\|\mathbf{H}_{d,M-1}\cdots\mathbf{H}_{d,2}(\sin(\omega\ \mathbf{H}_{d,1}v_d')) - \mathbf{H}_{d,M-1}\cdots\mathbf{H}_{d,2}(\sin(\omega\ \mathbf{H}_{d,1}v_d''))\|_{\ell_1}\\ &\leq\cdots\\ &\leq \eta^M\omega^{M-1}|v_d' - v_d''|,\end{aligned} \tag{34}$$

where $\{\mathbf{H}_{d,m}\}_{m=1}^M$ denote the weight matrices of $f_{\theta_d}(\cdot)$. Moreover, $\|\mathcal{C}_{l_1} - \mathcal{C}_{l_2}\|_{\ell_1} \leq 2\eta$. Combining the above inequalities, we have

$$\begin{aligned}&|s_{l_1}(v_1, v_2, \cdots, v_d', \cdots, v_{N+1}) - s_{l_2}(v_1, v_2, \cdots, v_d'', \cdots, v_{N+1})|\\ \leq&(\|\mathcal{C}_{l_1} - \mathcal{C}_{l_2}\|_{\ell_1}\|f_{\theta_d}(v_d')\|_{\ell_1} + \|\mathcal{C}_{l_2}\|_{\ell_1}\|f_{\theta_d}(v_d') - f_{\theta_d}(v_d'')\|_{\ell_1})\|f_{\theta_1}(v_1)\|_{\ell_1}\|f_{\theta_2}(v_2)\|_{\ell_1}\cdots\|f_{\theta_{N+1}}(v_{N+1})\|_{\ell_1}\\ \leq&(2\eta^{M+1}\omega^{M-1}\xi + \eta^{M+1}\omega^{M-1}|v_d' - v_d''|)\eta^{MN}\omega^{(M-1)N}\xi^N = \delta_1|v_d' - v_d''| + \delta_2,\end{aligned} \tag{35}$$

which concludes the inequality (30). When $l_1 = l_2$, we have $\|\mathcal{C}_{l_1} - \mathcal{C}_{l_2}\|_{\ell_1} = 0$ and the upper bound is

$$(\eta^{M+1}\omega^{M-1}|v_d' - v_d''|)\eta^{MN}\omega^{(M-1)N}\xi^N = \delta_1|v_d' - v_d''|. \tag{36}$$

The proof is completed. □

## REFERENCES

[1] Y. Luo, X. Zhao, Z. Li, M. K. Ng, and D. Meng, "Low-rank tensor function representation for multi-dimensional data recovery," *IEEE Transactions on Pattern Analysis and Machine Intelligence*, 2023, 10.1109/TPAMI.2023.3341688.

[2] T. G. Kolda and B. W. Bader, "Tensor decompositions and applications," *SIAM Review*, vol. 51, no. 3, pp. 455–500, 2009.
